# Supplementary material for: SDR: Efficient Neural Re-ranking using Succinct Document Representation
Source: arXiv:2110.02065 source file (2021-10-03)
Supplement: Supplementary file 1 [file appendix.tex]

\section{More analysis not in the paper}
\WIP{\amit{here to the end of the paper is WIP}
\nachshon{We can stop the paper here, and it might be helpful if we want to write another paper on analyzing how context affects word embedding vectors. }
\paragraph{Part-Of-Speech (POS) tag impact on reconstruction error} next, we consider how the role of a token affect its dependency on the context. 
Therefore, we run spacy\footnote{https://spacy.io/} to compute POS tagging over the document corpus we consider. 
For each token, we aggregate its POS \guy{It's a bit strange to talk about a token's POS} tag over all appearances in the documents. 
In this experiment, we only consider cases where most of the tokens (at least 2/3) share the same POS tag. 
Then, we compute the reconstruction error as a function of POS tag. 
In this experiment, we are less interested in the overall better quality of \ours{}. 
Therefore, to better understand the impact of POS tag on reconstruction error, we normalize it by dividing with the average reconstruction error on all tokens and reducing by 1. 
Therefore, a negative number means that the reconstruction error is lower than an average token (i.e., ``easy to reconstruct''), while a positive number means the reverse. 

Results are depicted in Figure~\ref{fig:analysis-pos}. 
We observe that AE and \oursabbr{} show very different behavior. 
AE demonstrate lower reconstruction rate for punctuation and determiner, average reconstruction error for prepositions, and high reconstruction error for nouns, verbs, adjectives, and proper nouns. 
In contrast, \oursabbr{} show lower reconstruction rate for nouns, verbs, adjectives, and proper nouns, but higher reconstruction rates for punctuation and prepositions, and much higher reconstruction rates for determiners. 
This behavior matches our expectation: determiners are stop words, which highly depend on the context, and as mentioned earlier, hard to reconstruct using the static token embedding. 
Similar phenomena happens also for punctuation and prepositions. \guy{I'm not sure the root cause here is that they "highly depend on the context", because we don't really understand what it is that BERT saves in those "contextualized" vectors of these kind of words. It is possible that while for more meaningful words the contextual embeddings are in fact contextual embeddings of the words, for the less meaningful words BERT uses the vectors to store some other information, which varies a lot from the initial embeddings and therefore is harder to reconstruct. Not sure how to deal with this but as a start maybe check similarity between the initial vectors and the contextual ones for different POS groups?} 
In contrast, nouns, verbs, adverbs, and proper nouns, all are very meaningful even without the context of a document. 
Therefore, for these cases, the reconstruction error of \oursabbr{} is much better than the average. 

\begin{figure}
	\centering
	\includegraphics[width=1.0\columnwidth]{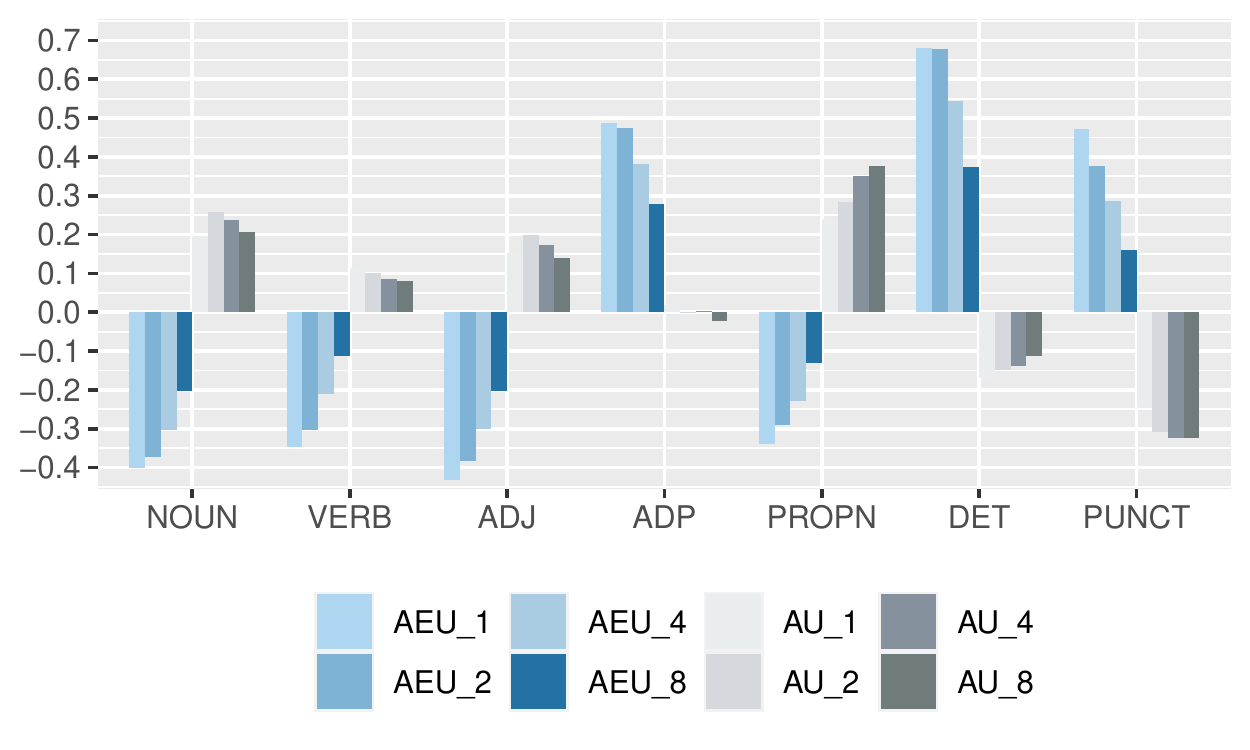}
	\caption{Normalized reconstruction error rate as a function of POS tag. Blue bars are \ours{}, while black bars are AE. Different shades imply different number of encoded dimension.}
	\label{fig:analysis-pos}
\end{figure}

\paragraph{Ambiguity impact on reconstruction error}
For humans, perhaps the most important factor in the context is the ability to disambiguate the meaning of a word. 
The word ``bank'' have two different meaning (geographical, institute), which are commonly disambiguate by providing some context, (``river bank'', ``bank of America''). 
Therefore, it is interesting to see if ambiguous tokens are harder to reconstruct based on the static token. 

Recall that in the POS experiment, we only consider tokens where the most frequent meaning cover at least 2/3 of the appearances of the token. 
We call such tokens non-ambiguous. 
We then consider tokens where the most frequent meaning does not cover 2/3 of the appearances of the token, and consider these ambiguous. \guy{I'm not sure this is a good definition for a couple of reasons: 1. a word might be "in POS ambiguous" and 2. number of appearances does not necessarily indicate number of meanings since language tends to be not evenly distributed (e.g. "duck" the animal (noun) is probably a lot more frequent than duck the verb. This might explain the unexpected results.}
We selected a subset of POS tags: nouns, verbs, adjectives, and proper nouns, for which there are many ambiguous and non-ambiguous tokens. 
For each POS tag, we compute the reconstruction error ratio between ambiguous tokens and non-ambiguous ones. 
This ratio minus one is the ambiguity impact: how much harder it is to reconstruct an ambiguous token compared to a non-ambiguous one, assuming that the most frequent interpretation has the same POS. 
Again, a negative score implies that an ambiguous token is easier to reconstruct compared to a non-ambiguous one. 
Unlike previous experiments, we show results for 12 and 16 floats, since they do not follow similar trends to 1, 2, 4, 8 floats we used in previous experiments.

Results appear in Figure~\ref{fig:analysis-ambiguity}. 
Except perhaps for proper nouns, differences are moderate and rarely bypass 15\% difference. 
This stands in contrast to our expectations that an ambiguous token would be much harder to reconstruct based on the static token and a few floats. 
Nevertheless, we do see that the ambiguity impact on \ours{} is larger than on a standard autoencoder. 
In addition, for the proper noun case, the impact of ambiguity is much stronger, reaching relatively high reconstruction rates for \ours{}, while being relatively easy to reconstruct for the autoencoder case. 
While we do not have an explanation for the exact phenomena, the overall results show that the static token embeddings is less effective for an ambiguous token compared to a non-ambiguous one. 

\begin{figure}
	\centering
	\includegraphics[width=3.2in]{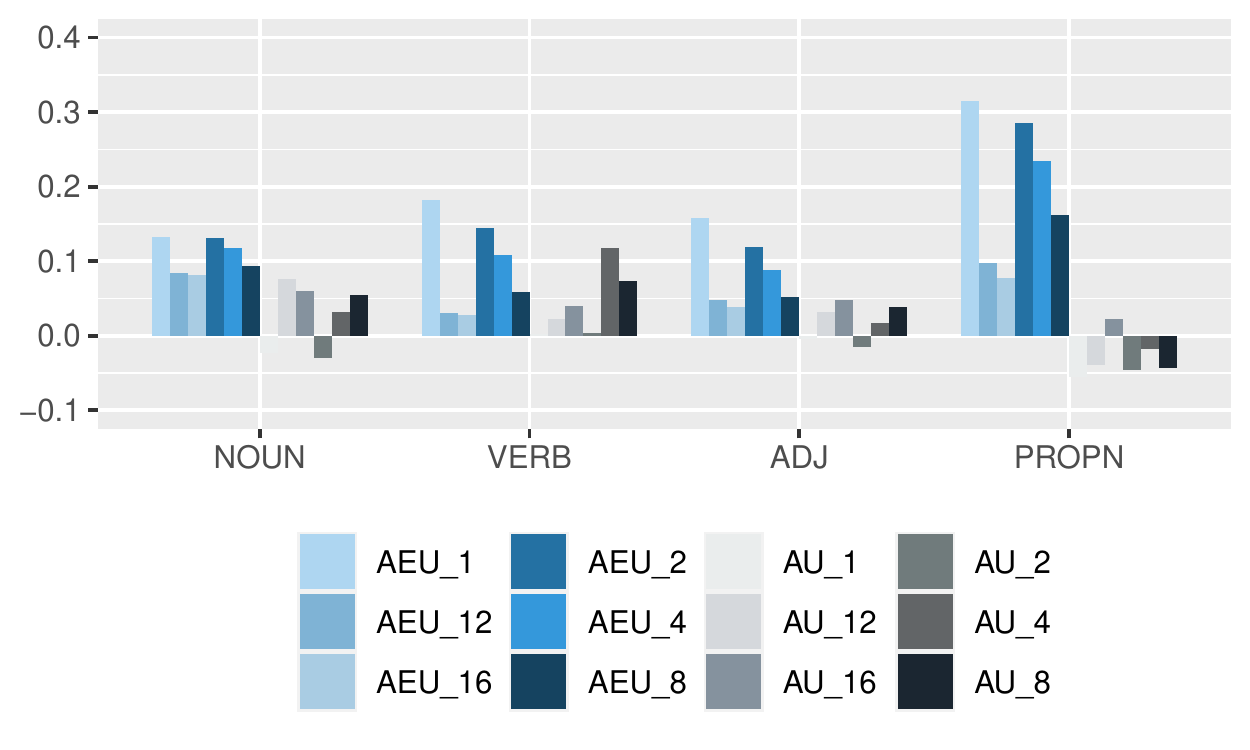}
	\caption{Reconstruction error rate vs. ambiguity. Labels are similar to Figure~\ref{fig:analysis-pos}. 
	\amit{color and order seems a bit confusing here and in figure 6, we may want to make sure that AEU/AU are ordered in the graph by number of feature and the brightness in the same scale}}
	\label{fig:analysis-ambiguity}
\end{figure}

}
